# Supplementary material for: DAL: Dynamic Angular Loss for Imbalanced Medical Image Classification
Source: arXiv:2611.24597 source file (2026-11-18)
Supplement: Supplementary file 2 [file appendix.tex]

\appendix
\newpage

\section{Implementation Details}
\label{appx:implementation}


All models are implemented in PyTorch \cite{paszke2019pytorch} using a ResNet-18 backbone~\cite{he2016deep} pre-trained on ImageNet \cite{russakovsky2015imagenet}. 
Following \citet{deng2022arcface}, we replace the original fully connected layer with a lightweight two-layer classification head consisting of a dropout layer, a linear projection from the 512-dimensional backbone output to a 128-dimensional embedding, followed by Batch Normalization which is fed to our classification layer. 
For baseline models, we use ReLU layer instead of Batch Normalization and a final linear layer producing $C$ outputs. 
All images are resized to $224 \times 224$, and training is performed using stochastic gradient descent (SGD) with a learning rate of $0.001$, momentum of $0.9$, and weight decay of $0.0001$. 
A batch size of 128 is used, and each model is trained for 30 epochs. 
To stabilize optimization, the ResNet-18 backbone is frozen for the first five epochs so that only the classification head is updated; thereafter, all layers are fine-tuned jointly. 
For every dataset, we follow the train/validation/test protocol described previously and select the checkpoint that achieves the highest balanced accuracy on the validation set.


\section{Ablation Study of our Method}
\label{appx:ablation}
\input{tables/hyperparameters}
To better understand the influence of ArcFace design choices under severe class imbalance, \tabref{tab:isic2018hyperparameters} evaluates a wide range of scale values $s$, margin values $m$, and the presence or absence of dynamic weighted cross-entropy (DWCE) on ISIC 2018. 
A clear trend emerges: models trained without DWCE consistently underperform those trained with DWCE, demonstrating that explicit imbalance compensation remains crucial for reliable decision boundaries. 
\textcolor{blue}{Especially, we can see that when the model is trained with just DWCE without angular constraints, we get a huge boost in results in all the metrics. When we combine the angular loss with DWCE, the results improve by about 4\% showing that angular loss requires some form of reweighting to tackle the huge class imbalance problem and reinforces the conclusion from \secref{sec:combining} of the main paper.}

\begin{figure}[t]
\floatconts{fig:softmax-distribution}
{\color{blue}\Caption{Softmax Probability Distribution}{
    We show the probability distributions of \subfigref{fig:distributions-positive} the correct classes and \subfigref{fig:distributions-negative} the highest incorrect class scores per sample on the ISIC 2018 test set for models trained with the scale value $s=2.56$ obtained via \eqref{eq:adacos-s} and our proposed $s=4$, both applied with no margin.
}}
{
\subfigure[\textcolor{blue}{Correct Class Probabilities}]{\label{fig:distributions-positive}
\includegraphics[width=.45\textwidth]{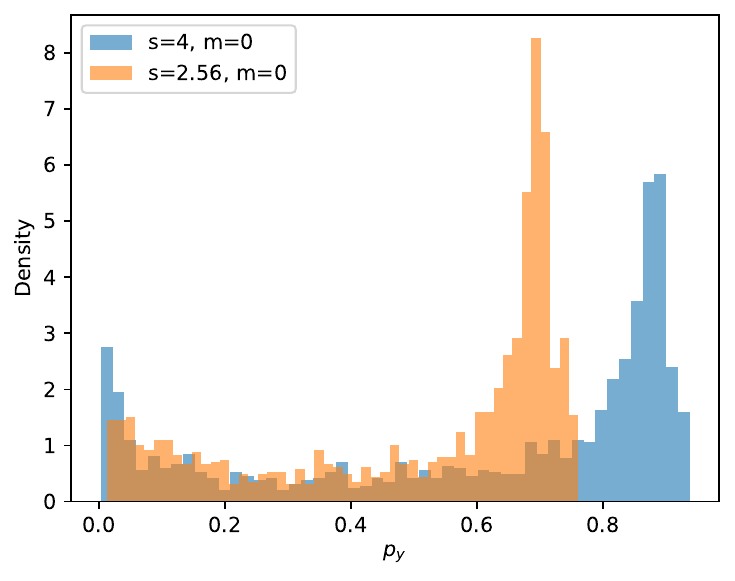}
}
\hfill
\subfigure[\textcolor{blue}{Incorrect Class Probabilities}]{\label{fig:distributions-negative}
\includegraphics[width=.45\textwidth]{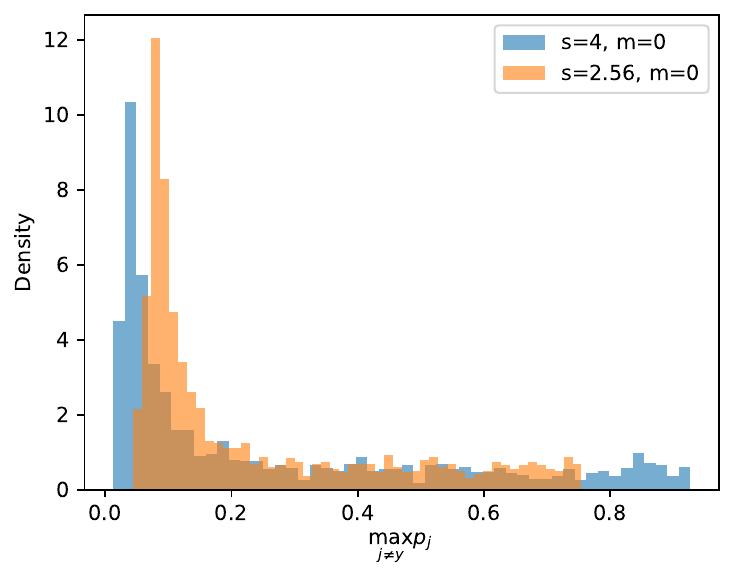}
}}
\end{figure}

Additionally, the results indicate that large values of $s$ or $m$ are not beneficial in this setting, likely due to the difficulty of optimizing angular constraints when class distributions are highly uneven. However, we do observe that for larger values of $s$, relatively larger $m$ perform better than lower ones. 
\textcolor{blue}{When comparing the fixed AdaCos scale $s=2.56$ derived via \eqref{eq:adacos-s} with our chosen scale $s = 4$, we observe that selecting a reasonable scale value leads to stable behavior when combined with DWCE, while having little impact on overall classification performance as long as the scale is not excessively large. 
In practice, performance remains largely similar across a range of reasonable scale values, including the fixed AdaCos setting. At the same time, using $s = 4$ yields modest improvements (approximately 3\%) in Accuracy and Macro-F1, indicating a slightly more favorable operating point without altering the overall performance trend.}

\textcolor{blue}{\figref{fig:softmax-distribution} illustrates the softmax probability distributions on the test set $s=2.56$ and $s = 4$. 
Although both settings achieve comparable classification performance, the lower $s=2.56$ produces systematically under-confident probability estimates, with predicted probabilities rarely exceeding 0.8 and most values concentrated around 0.7. In contrast, the model trained with $s = 4$ yields higher-confidence predictions, including probabilities approaching 1.0. This behavior reflects a calibration effect rather than a change in ranking performance.
}

Overall, our selected configuration, which combines a moderate angular parameterization with DWCE, achieves the strongest balanced metrics. \textcolor{blue}{While the proposed batch-adaptive angular margin (BAAM) provides additional refinement, its contribution is comparatively modest. In practice, BAAM primarily affects a small subset of borderline samples by enforcing a stricter angular separation during training, leading to marginal but consistent improvements in certain cases. These results indicate that BAAM plays a secondary, complementary role, whereas imbalance-aware optimization via DWCE with a reasonable scale parameter remains the dominant factor driving performance gains.}
These improvements are further confirmed to be statistically significant based on a paired t-test for balanced accuracy, compared against all listed baseline variants.


\section{Validation Set Evaluation}
\label{appx:validation}

\input{tables/performace_validation}

\tabref{tab:validation-results} summarizes the validation set results on the ISIC 2018 and ISIC 2019 datasets, averaged over five independent runs. 
As opposed to the test set reported in the main paper, the validation set is not split by patient, so different lesions of the same patient may appear in the training and validation sets.
This mimics the evaluation setup as performed by \citet{yue2022toward}.
It is interesting to note that, on the validation set, AWB loss and PF loss perform quite competitively compared to our method for the ISIC 2018 dataset, and even surpass its performance on ISIC 2019. 
However, as shown in \tabref{tab:test-results}, this performance advantage does not translate to the identity-disjoint test sets of ISIC 2018 and ISIC 2019.

\input{tables/perclass_validation}

\tabref{tab:perclass-validation} presents the per-class recall for both ISIC 2018 and ISIC 2019, averaged over five independent runs, and provides a closer look into the performance of each class on the validation set. 
A closer inspection reveals that the validation set improvements for the minority classes do not carry over to the test set, as demonstrated in \tabref{tab:perclass}. For example, we observe a significant performance gap in the minority-class TPR on the test sets compared to the validation sets, especially for AWB loss, where the gap is considerably larger. 
In contrast, PF loss generalizes better from validation to test sets compared to AWB. 
Although our method underperforms compared to AWB loss on the ISIC 2019 validation results, the test set performance clearly shows that it generalizes more effectively to unseen patients. 
This suggests that AWB loss may be overfitting to the training set, likely due to data leakage or noise in the dataset, whereas our method learns more discriminative features and achieves stronger generalization. 
The remaining loss functions primarily benefit the majority classes. 

\input{tables/isic-2018-confusion}
\input{tables/isic-2019-confusion}

To provide more thorough insight into performance differences, \figref{fig:isic2018_cm_all_losses} and \figref{fig:isic2019_cm_all_losses} show the confusion matrices for all loss functions using the best-performing model over five independent runs on the test sets of ISIC 2018 and ISIC 2019, respectively. 
We do not report further evaluation metrics for the APTOS dataset, as it does not include a predefined test set and, therefore, test-set generalization cannot be reliably assessed.


\section{Negative Angle Distributions}
\label{appx:angles}
In \figref{fig:negative-angles-s4} in the main paper, we have shown how the distribution of negative angles evolve over time, with a fixed parameter of $s=4$.
Using this distribution, we performed a theoretical analysis and to arrive at an optimal value for $s=4$.
We acknowledge that this is a chicken/egg problem, and there is a possibility that other parameters of $s$ yield substantially different angle distributions.
Therefore, we performed the same analysis for other $s$ parameters in \figref{fig:negative_angles_s_scales} to show that the distribution of negative angles $\theta_{i,j}$ is mostly independent of the actual $s$ parameter, so even if we would have started our analysis with a larger $s$ value, we would have arrived at similar theoretical bounds and optimum value for $s$.

\input{tables/distributions-s}

\section{Effect of Margin}
\label{appx:margin}
\begin{figure}[t]
\floatconts{fig:margin}
{\color{blue}\Caption{Effect of angular margin on softmax probabilities}{
This figure illustrates the effect of introducing an angular margin ($m=0.2$) on the softmax probability distribution compared to the no-margin case ($m=0$) for $s=4$.
Color coding is identical to \figref{fig:arcface-s-comparison} in the main paper.
}}
{\includegraphics[width=0.75\linewidth]{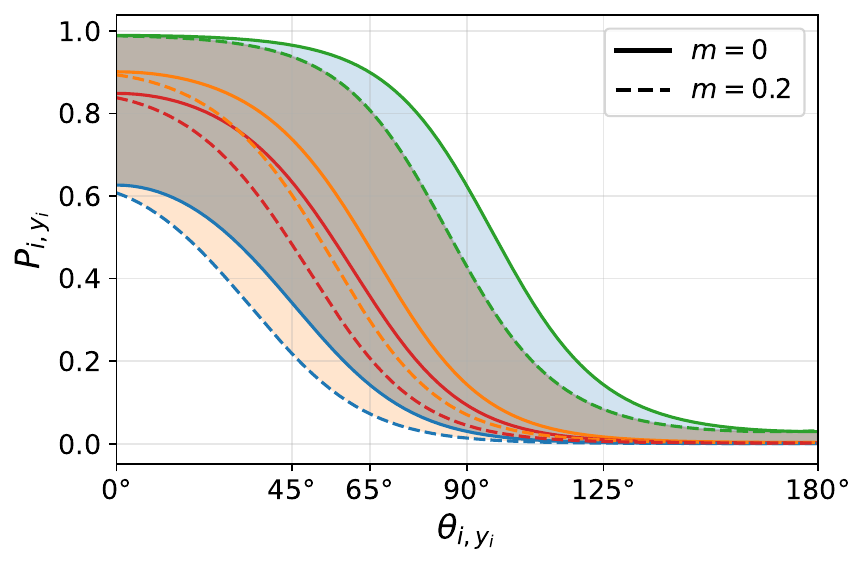}\vspace*{-4ex}}
\end{figure}

\textcolor{blue}{
\figref{fig:margin} shows the effect of introducing an angular margin on the softmax probability curves for a fixed scale value of $s=4$. In our experiments, the maximum margin applied is $m=0.2$. 
As observed, adding a margin leads to a small shift in the probability curves, while the overall shape and spread of the distributions remain largely unchanged. 
This indicates that the margin primarily modifies the decision strictness during training rather than substantially altering the resulting probability distribution. 
In the proposed batch-adaptive angular margin, smaller margins are assigned to most classes, with slightly larger margins applied to a limited number of minority classes. 
Consequently, the overall influence of the margin on the probability distribution is limited, which is consistent with the modest differences observed between the margin and no-margin cases in \tabref{tab:isic2018hyperparameters}.
These results suggest that the margin plays a secondary role relative to other components of the method.
}





% This is a complete version of a proof sketched in the main text.
